# Supplementary material for: Interpolation for Robust Learning: Data Augmentation on Wasserstein Geodesics
Source: arXiv:2302.02092 source file (2023-08-28)
Supplement: Supplementary file 1 [file batch_PCA.tex]

\begin{tabular}{cc|ccccccccccc}
    \toprule
      $\sigma$ & Batch (MNIST)   & 0.00 & 0.25 & 0.50 & 0.75 & 1.00 & 1.25 & 1.50 & 1.75 & 2.00 & 2.25 & 2.50  \\ 
    \midrule
     \multirow{7.5}{*}{0.5} 
     &8 &98.60	&97.50 &	96.10	&94.10	&89.70 	&82.50	&69.30	&50.30	&0.00	&0.00	&0.00	\\
    &16 &99.10	&98.30 &97.40	&95.30	&92.20	&85.90	&74.80	&56.70	&0.00	&0.00	&0.00	\\
    &32 &99.10	&98.10	&97.10	&95.70	&91.40	&86.10	&74.40	&57.40	&0.00	&0.00	&0.00	\\
    &64 &99.20	&98.30	&97.20	&95.50	&92.00 &85.50	&74.90	&58.30	&0.00	&0.00	&0.00	\\
    &128 &99.20	&98.10	&97.20&	95.10	&91.30	&85.10	&74.60	&55.90	&0.00 &	0.00	&0.00	\\
    &256 &99.00	&98.40	&96.90	&95.30	&91.20	&84.80&	73.60	&55.40&	0.00&	0.00	&0.00	\\
    & 512 &99.10	&98.00	&96.60	&94.10	&89.80	&84.00	&71.50	&52.90	&0.00	&0.00	&0.00 \\
    \bottomrule
\end{tabular}
