# Supplementary material for: Interpolation for Robust Learning: Data Augmentation on Wasserstein Geodesics
Source: arXiv:2302.02092 source file (2023-08-28)
Supplement: Supplementary file 2 [file batch_VAE.tex]

\begin{tabular}{cc|ccccccccccc}
    \toprule
      $\sigma$ & Batch (MNIST)   & 0.00 & 0.25 & 0.50 & 0.75 & 1.00 & 1.25 & 1.50 & 1.75 & 2.00 & 2.25 & 2.50  \\ 
    \midrule
     \multirow{7.5}{*}{0.5} 
     &8 &99.00&	97.70	&96.40	&94.40	&90.60&82.30&	68.00	&46.70	&0.00	&0.00	&0.00	\\
    &16 &98.70&	97.70&	96.50&94.90&	91.00	&83.20&	70.30	&50.50	&0.00	&0.00	&0.00	\\
    &32 &98.70&	97.70&	96.60	&94.90	&90.90	&83.80	&72.40	&52.20	&0.00	&0.00	&0.00	\\
    &64 &98.80	&97.60	&96.50&95.00&	91.40&	83.20	&71.30	&51.40	&0.00	&0.00	&0.00	\\
    &128 &99.00	&97.30&	96.50&	95.00	&90.70	&84.20&	70.80&51.50	&0.00 &	0.00	&0.00	\\
    &256 &98.50	&97.30&	96.40&	94.90	&90.30	&83.10	&70.00&	49.20 &	0.00&	0.00	&0.00	\\
    & 512 &98.60	&97.40	&96.10	&94.20	&89.80	&81.90	&69.00	&50.30	&0.00	&0.00	&0.00 \\
    \bottomrule
\end{tabular}
