# Supplementary material for: Interpolation for Robust Learning: Data Augmentation on Wasserstein Geodesics
Source: arXiv:2302.02092 source file (2023-08-28)
Supplement: Supplementary file 4 [file mixY_PCA_0.5.tex]

\begin{tabular}{cc|ccccccccccc}
    \toprule
      $\sigma$ & $t$ (MNIST)  & 0.00 & 0.25 & 0.50 & 0.75 & 1.00 & 1.25 & 1.50 & 1.75 & 2.00 & 2.25 & 2.50  \\ 
    \midrule
     \multirow{4}{*}{0.5} 
&0.1 &98.10	&96.90	&95.70	&93.70	&90.20	&84.70	&76.60	&64.20	&0.00	&0.00	&0.00\\	
&0.2 &98.20	&97.20	&95.00	&92.50	&88.90	&83.50	&75.80	&61.40	&0.00	&0.00	&0.00	\\
&0.3 &98.20 &	96.90	&95.60	&94.10	&89.70	&84.70	&76.20 & 	62.40	&0.00	&0.00	&0.00	\\
&0.4 &98.10	&96.60	&95.20	&93.20	&89.60	&85.20	&76.50	&62.70	&0.00	&0.00	&0.00	\\
    \bottomrule
\end{tabular}
