# Supplementary material for: Interpolation for Robust Learning: Data Augmentation on Wasserstein Geodesics
Source: arXiv:2302.02092 source file (2023-08-28)
Supplement: Supplementary file 5 [file mixY_PCA_1.0.tex]

\begin{tabular}{cc|ccccccccccc}
    \toprule
      $\sigma$ & $t$ (MNIST)  & 0.00 & 0.25 & 0.50 & 0.75 & 1.00 & 1.25 & 1.50 & 1.75 & 2.00 & 2.25 & 2.50  \\ 
    \midrule
     \multirow{4}{*}{1.0} 
&0.1 &87.50	&83.40	&78.20	&72.60	&65.50	&59.40	&52.20	&45.20&	40.60&	35.20	&29.90	\\
&0.2 &90.10	&87.70&	83.60	&77.10&	69.90	&63.60	&54.50	&44.50&	35.30&	27.60	&19.10	\\
&0.3 &87.60	&84.00	&78.90	&71.80&	64.90&	58.80	&50.70	&43.80	&37.70	&32.40	&26.50	\\
&0.4 &86.80	&82.50&	78.10&	73.30	&66.70&	58.50	&52.30&	45.00	&38.40	&32.00	&26.30 \\	
    \bottomrule
\end{tabular}
