# Supplementary material for: Interpolation for Robust Learning: Data Augmentation on Wasserstein Geodesics
Source: arXiv:2302.02092 source file (2023-08-28)
Supplement: Supplementary file 6 [file mixY_VAE_0.25.tex]

\begin{tabular}{cc|ccccccccccc}
    \toprule
      $\sigma$ & $t$ (MNIST)  & 0.00 & 0.25 & 0.50 & 0.75 & 1.00 & 1.25 & 1.50 & 1.75 & 2.00 & 2.25 & 2.50  \\ 
    \midrule
     \multirow{4}{*}{0.25} 
&0.1 &99.00	&98.10	&97.50	&95.80	&0.00	&0.00	&0.00	&0.00	&0.00	&0.00	&0.00\\	
&0.2 &99.00	&98.10	&97.30	&95.80			&0.00	&0.00	&0.00	&0.00	&0.00	&0.00	&0.00	\\
&0.3 &98.80	&98.10	&97.30	&96.00	&0.00	&0.00	&0.00	&0.00	&0.00	&0.00	&0.00\\
&0.4 &98.70	&98.00	&97.30	&95.80		&0.00	&0.00	&0.00	&0.00	&0.00	&0.00	&0.00	\\
    \bottomrule
\end{tabular}
