# Supplementary material for: Interpolation for Robust Learning: Data Augmentation on Wasserstein Geodesics
Source: arXiv:2302.02092 source file (2023-08-28)
Supplement: Supplementary file 7 [file mixY_VAE_0.5.tex]

\begin{tabular}{cc|ccccccccccc}
    \toprule
      $\sigma$ & $t$ (MNIST)  & 0.00 & 0.25 & 0.50 & 0.75 & 1.00 & 1.25 & 1.50 & 1.75 & 2.00 & 2.25 & 2.50  \\ 
    \midrule
     \multirow{4}{*}{0.5} 
&0.1 &97.80	&96.90	&96.20	&94.30	&91.70	&87.70	&78.70	&67.10	&0.00	&0.00	&0.00\\	
&0.2 &97.90	&97.10	&96.00	&94.30	&91.90	&87.80	&79.50	&66.50	&0.00	&0.00	&0.00	\\
&0.3 &97.80	&97.10	&96.10	&94.00	&91.90	&86.80	&78.90	&67.10	&0.00	&0.00	&0.00	\\
&0.4 &97.90	&97.10	&96.20	&94.10	&91.40	&86.40	&78.00 &	66.40		&0.00	&0.00	&0.00	\\
    \bottomrule
\end{tabular}
