# Supplementary material for: Interpolation for Robust Learning: Data Augmentation on Wasserstein Geodesics
Source: arXiv:2302.02092 source file (2023-08-28)
Supplement: Supplementary file 8 [file mixY_VAE_1.0.tex]

\begin{tabular}{cc|ccccccccccc}
    \toprule
      $\sigma$ & $t$ (MNIST)  & 0.00 & 0.25 & 0.50 & 0.75 & 1.00 & 1.25 & 1.50 & 1.75 & 2.00 & 2.25 & 2.50  \\ 
    \midrule
     \multirow{4}{*}{1.0} 
&0.1 &91.50	&88.90	&85.10	&81.80	&75.80	&68.50	&61.30	&52.20	&44.60	&37.20	&29.80	
	\\
&0.2 &91.70	&88.30&85.40&	80.50	&75.40&	67.90	&61.20	&52.20	&44.00	&37.70	&30.60	
	\\
&0.3& 90.80&	88.50&	85.80	&81.20	&75.50&	67.40&	60.20	&51.70&	43.50	&34.90	&28.70	
	\\
&0.4 &91.00	&88.40	&85.30	&80.80	&75.40	&67.20	&59.30	&51.00	&43.00	&34.60	&28.80 \\	
    \bottomrule
\end{tabular}
